# Supplementary material for: The Role of Context in Detecting Previously Fact-Checked Claims
Source: arXiv:2104.07423 source file (2022-05-09)
Supplement: Supplementary file 1 [file supplemental_material.tex]

\section{Experimental Details}

\paragraph{Hyper-parameters}

$FC(3,1)$:

top-3 sentences

top-100 sentences

pre-training on FEVER, 

\textbf{Rank-SVM:}  

\textbf{BM25}\cite{robertson2009probabilistic}: It is a classical approach in information retrieval. It assigns a score to each query-document pair based on exact matching between the words in the query and the words in a target document, and it uses this score for ranking.
